# Supplementary material for: Subset Representations and Eigenvalues of the Universal Intertwining Matrix
Source: arXiv:2011.02942 ancillary file (2021-03-06)
Supplement: Supplementary file 1 [file Combi.pdf]

Proof of our formula for the sum  
over  $j$ ,  $p$  of the  
 $(-1)^{(k-j)} \text{Binomial}[k, j]$   
 $\text{Binomial}[m-j, p]$   
 $\text{Binomial}[m+j-k, j+p]$   
 $b[p+j]$ , when  
 $b[m] = (-1)^m (2m)!! / (2m-1)!!$

---

We use a RISC package from Linz.

```
In[1]:= ClearAll[Evaluate[Context[] <> "*"]]
```

```
In[2]:= << RISC/MultiSum.m
```

Package MultiSum version 2.3 written by Kurt Wegschaider  
enhanced by Axel Riese and Burkhard Zimmermann  
Copyright Research Institute for Symbolic Computation (RISC),  
Johannes Kepler University, Linz, Austria

```
In[3]:= w[k_] := (-1) ^ (m - k) (2 k - 1) !! (2 m - 2 k) !! / ((2 m - 1) !!)
```

```
In[4]:= Table[w[p - 1] == - (2 m + 2 - 2 p) / (2 p - 1) w[p], {m, 4}, {p, m}]
```

```
Out[4]:= {{True}, {True, True}, {True, True, True}, {True, True, True, True}}
```

---

Their package does not deal with double factorials, so  
we use Gamma functions instead.

```
In[5]:= x[k_] := (-1) ^ (k) 
$$\frac{\text{Gamma}\left[\frac{1}{2} + m - k\right] \text{Gamma}[1 + k]}{\text{Gamma}\left[\frac{1}{2} + m\right]}$$

```

```
In[6]:= x[k_, m_] := (-1) ^ (k) 
$$\frac{\text{Gamma}\left[\frac{1}{2} + m - k\right] \text{Gamma}[1 + k]}{\text{Gamma}\left[\frac{1}{2} + m\right]}$$

```

```
In[7]:= Table[w[p] == x[m - p], {m, 4}, {p, 0, m}]
```

```
Out[7]= {{True, True}, {True, True, True},  
         {True, True, True, True}, {True, True, True, True, True}}
```

Because of the pole in  $b[p+j]=x[p+j,m]$  at negative  $p+j$  we now put

```
In[8]:= x[k_?Negative, m_] := 0;
```

We need to break an ambiguity in Binomial.

```
In[9]:= Binomial[k, -2]
```

```
Out[9]= 0
```

```
In[10]:= Binomial[-2, -2]
```

```
Out[10]= 1
```

We follow the conventions of the A=B book.

```
In[11]:= binomial[m_, k_] := Binomial[m, k];  
         binomial[m_, k_?Negative] := 0;
```

The main term

```
In[13]:= f[m_, k_, j_, p_] :=  
         (-1) ^ (k - j) binomial[k, j] × binomial[m - j, p] × binomial[m + j - k, j + p] × x[p + j, m]
```

If  $m \geq k \geq 0$ , then  $f[m, k, j, p]$  vanishes unless  $0 \leq p \leq m - k$ ,  $0 \leq j \leq k$ .

In[14]:= ? Delta

Symbol

Delta[k, expr] denotes the forward shift difference operator given by  $\Delta[k, \text{expr}] := (\text{expr} /. k \rightarrow k+1) - \text{expr}$ .

In GeneratingFunctions, Delta[A] gives the forward difference of sequence A, i.e. a sequence, where the  $n$ -th element contains  $a[n+1] - a[n]$  and  $a[n]$  is the  $n$ -th element in the sequence A, which has been defined by the procedure DefineSequence.

In HolonomicFunctions, Delta[var] denotes the Ore operator "forward difference w.r.t. var".

In[15]:= recf = FindRecurrence[f[m, k, j, p], {m, k}, {j, p}]

Out[15]:= 
$$\begin{aligned} & \{ 4 (-3 + k) (-2 + k) (-3 + 2m) F[-3 + m, -4 + k, -2 + j, -1 + p] + \\ & \quad 4 (-2 + k) (-5 + 2m) (-4 + k + 2m) F[-2 + m, -3 + k, -2 + j, -1 + p] + \\ & \quad (-5 + 2m) (-3 + 2m) (-7 + 4k + 2m) F[-1 + m, -2 + k, -2 + j, -1 + p] + \\ & \quad (-5 + 2m) (-3 + 2m) (-1 + 2m) F[m, -1 + k, -2 + j, -1 + p] = \\ & \Delta_j [-4 (-2 + k) (-3 + k + m) (-5 + 2m) F[-2 + m, -3 + k, -2 + j, p] + \\ & \quad 4 (-1 + k - m) (-1 + m) (-5 + 2m) F[-2 + m, -2 + k, -2 + j, -1 + p] - \\ & \quad 4 (-1 + k - m) (-1 + m) (-5 + 2m) F[-2 + m, -2 + k, -2 + j, p] - \\ & \quad (-5 + 2m) (-3 + 2m) (-7 + 4k + 2m) F[-1 + m, -2 + k, -2 + j, p] - \\ & \quad (-3 + 2k) (-5 + 2m) (-3 + 2m) F[-1 + m, -2 + k, -1 + j, p] + \\ & \quad 2 (-1 + k - m) (-5 + 2m) (-3 + 2m) F[-1 + m, -1 + k, -2 + j, -1 + p] - \\ & \quad 2 (-1 + k - m) (-5 + 2m) (-3 + 2m) F[-1 + m, -1 + k, -2 + j, p] + \\ & \quad 2 (-1 + k - m) (-5 + 2m) (-3 + 2m) F[-1 + m, -1 + k, -1 + j, -1 + p] - \\ & \quad 2 (-1 + k - m) (-5 + 2m) (-3 + 2m) F[-1 + m, -1 + k, -1 + j, p] - \\ & \quad (-5 + 2m) (-3 + 2m) (-1 + 2m) F[m, -1 + k, -2 + j, p] - \\ & \quad (-5 + 2m) (-3 + 2m) (-1 + 2m) F[m, -1 + k, -1 + j, p] ] + \\ & \Delta_p [-4 (-3 + k) (-2 + k) (-3 + 2m) F[-3 + m, -4 + k, -2 + j, -1 + p] - \\ & \quad 4 (-2 + k) (-5 + 2m) (-4 + k + 2m) F[-2 + m, -3 + k, -2 + j, -1 + p] - \\ & \quad 4 (-1 + k - m) (-1 + m) (-5 + 2m) F[-2 + m, -2 + k, -2 + j, -1 + p] - \\ & \quad (-5 + 2m) (-3 + 2m) (-7 + 4k + 2m) F[-1 + m, -2 + k, -2 + j, -1 + p] - \\ & \quad 2 (-1 + k - m) (-5 + 2m) (-3 + 2m) F[-1 + m, -1 + k, -2 + j, -1 + p] - \\ & \quad (-5 + 2m) (-3 + 2m) (-1 + 2m) F[m, -1 + k, -2 + j, -1 + p] ], \\ & -4 (-3 + k) (-2 + k) (-1 + k) (-3 + 2m) F[-3 + m, -4 + k, -2 + j, -1 + p] - \\ & \quad 4 (-2 + k) (-1 + k) (-3 + k + m) (-5 + 2m) F[-2 + m, -3 + k, -2 + j, -1 + p] - \\ & \quad 4 (-1 + k) (k - 2m) (-1 + m) (-5 + 2m) F[-2 + m, -2 + k, -2 + j, -1 + p] - \\ & \quad (-1 + k) (-3 + 4k - 2m) (-5 + 2m) (-3 + 2m) F[-1 + m, -2 + k, -2 + j, -1 + p] + \\ & \quad 4 (-1 + m) m (-5 + 2m) (-3 + 2m) F[-1 + m, -1 + k, -2 + j, -1 + p] - \end{aligned}$$

$$\begin{aligned}
& (k-m)(-5+2m)(-3+2m)(-1+2m)F[m, -1+k, -2+j, -1+p] + \\
& (-1+m)(-5+2m)(-3+2m)(-1+2m)F[m, k, -2+j, -1+p] = \\
\Delta_j & \left[ 4(-2+k)(-1+k)(-3+k+m)(-5+2m)F[-2+m, -3+k, -2+j, p] - \right. \\
& 4(-1+k)(-1+m)^2(-5+2m)F[-2+m, -2+k, -2+j, -1+p] + \\
& 4(-1+k)(-1+k-m)(-1+m)(-5+2m)F[-2+m, -2+k, -2+j, p] + \\
& (-1+k)(-3+4k-2m)(-5+2m)(-3+2m)F[-1+m, -2+k, -2+j, p] + \\
& (-1+k)(-3+2k)(-5+2m)(-3+2m)F[-1+m, -2+k, -1+j, p] - \\
& 2(-5+2m)(-3+2m)(1-2k+k^2-km+m^2)F[-1+m, -1+k, -2+j, -1+p] + \\
& 2(-5+2m)(-3+2m)(1-2k+k^2+2m-km-m^2)F[-1+m, -1+k, -2+j, p] - \\
& 2(-5+2m)(-3+2m)(1-2k+k^2-km+m^2)F[-1+m, -1+k, -1+j, -1+p] + \\
& 2(-1+k)(-1+k-m)(-5+2m)(-3+2m)F[-1+m, -1+k, -1+j, p] + \\
& (k-m)(-5+2m)(-3+2m)(-1+2m)F[m, -1+k, -2+j, p] + \\
& (k-m)(-5+2m)(-3+2m)(-1+2m)F[m, -1+k, -1+j, p] - \\
& (-1+m)(-5+2m)(-3+2m)(-1+2m)F[m, k, -2+j, p] - \\
& \left. (-1+m)(-5+2m)(-3+2m)(-1+2m)F[m, k, -1+j, p] \right] + \\
\Delta_p & \left[ 4(-3+k)(-2+k)(-1+k)(-3+2m)F[-3+m, -4+k, -2+j, -1+p] + \right. \\
& 4(-2+k)(-1+k)(-3+k+m)(-5+2m)F[-2+m, -3+k, -2+j, -1+p] + \\
& 4(-1+k)(-1+k-m)(-1+m)(-5+2m)F[-2+m, -2+k, -2+j, -1+p] + \\
& (-1+k)(-3+4k-2m)(-5+2m)(-3+2m)F[-1+m, -2+k, -2+j, -1+p] + \\
& 2(-5+2m)(-3+2m)(1-2k+k^2+2m-km-m^2)F[-1+m, -1+k, -2+j, -1+p] + \\
& (k-m)(-5+2m)(-3+2m)(-1+2m)F[m, -1+k, -2+j, -1+p] - \\
& \left. (-1+m)(-5+2m)(-3+2m)(-1+2m)F[m, k, -2+j, -1+p] \right] \}
\end{aligned}$$

---

It found two recurrences. We take the first one.

In[16]:= `recf[[1]]`

```

Out[16]= 4 (-3 + k) (-2 + k) (-3 + 2 m) F[-3 + m, -4 + k, -2 + j, -1 + p] +
  4 (-2 + k) (-5 + 2 m) (-4 + k + 2 m) F[-2 + m, -3 + k, -2 + j, -1 + p] +
  (-5 + 2 m) (-3 + 2 m) (-7 + 4 k + 2 m) F[-1 + m, -2 + k, -2 + j, -1 + p] +
  (-5 + 2 m) (-3 + 2 m) (-1 + 2 m) F[m, -1 + k, -2 + j, -1 + p] ==
  Δj [-4 (-2 + k) (-3 + k + m) (-5 + 2 m) F[-2 + m, -3 + k, -2 + j, p] +
  4 (-1 + k - m) (-1 + m) (-5 + 2 m) F[-2 + m, -2 + k, -2 + j, -1 + p] -
  4 (-1 + k - m) (-1 + m) (-5 + 2 m) F[-2 + m, -2 + k, -2 + j, p] -
  (-5 + 2 m) (-3 + 2 m) (-7 + 4 k + 2 m) F[-1 + m, -2 + k, -2 + j, p] -
  (-3 + 2 k) (-5 + 2 m) (-3 + 2 m) F[-1 + m, -2 + k, -1 + j, p] +
  2 (-1 + k - m) (-5 + 2 m) (-3 + 2 m) F[-1 + m, -1 + k, -2 + j, -1 + p] -
  2 (-1 + k - m) (-5 + 2 m) (-3 + 2 m) F[-1 + m, -1 + k, -2 + j, p] +
  2 (-1 + k - m) (-5 + 2 m) (-3 + 2 m) F[-1 + m, -1 + k, -1 + j, -1 + p] -
  2 (-1 + k - m) (-5 + 2 m) (-3 + 2 m) F[-1 + m, -1 + k, -1 + j, p] -
  (-5 + 2 m) (-3 + 2 m) (-1 + 2 m) F[m, -1 + k, -2 + j, p] -
  (-5 + 2 m) (-3 + 2 m) (-1 + 2 m) F[m, -1 + k, -1 + j, p]] +
  Δp [-4 (-3 + k) (-2 + k) (-3 + 2 m) F[-3 + m, -4 + k, -2 + j, -1 + p] -
  4 (-2 + k) (-5 + 2 m) (-4 + k + 2 m) F[-2 + m, -3 + k, -2 + j, -1 + p] -
  4 (-1 + k - m) (-1 + m) (-5 + 2 m) F[-2 + m, -2 + k, -2 + j, -1 + p] -
  (-5 + 2 m) (-3 + 2 m) (-7 + 4 k + 2 m) F[-1 + m, -2 + k, -2 + j, -1 + p] -
  2 (-1 + k - m) (-5 + 2 m) (-3 + 2 m) F[-1 + m, -1 + k, -2 + j, -1 + p] -
  (-5 + 2 m) (-3 + 2 m) (-1 + 2 m) F[m, -1 + k, -2 + j, -1 + p]]

```

---

We may check the recurrence, and do not need the RISC package for that. We first define lhsf, ..

```
In[17]:= recf[[1, 1]] /. m → m - 1 // Simplify
```

```

Out[17]= 4 (-3 + k) (-2 + k) (-5 + 2 m) F[-4 + m, -4 + k, -2 + j, -1 + p] +
  4 (-2 + k) (-7 + 2 m) (-6 + k + 2 m) F[-3 + m, -3 + k, -2 + j, -1 + p] +
  (-7 + 2 m) (-5 + 2 m) (-9 + 4 k + 2 m) F[-2 + m, -2 + k, -2 + j, -1 + p] +
  (-7 + 2 m) (-5 + 2 m) (-3 + 2 m) F[-1 + m, -1 + k, -2 + j, -1 + p]

```

```

In[18]:= lhsf = 4 (-3 + k) (-2 + k) (-5 + 2 m) F[-4 + m, -4 + k, -2 + j, -1 + p] +
  4 (-2 + k) (-7 + 2 m) (-6 + k + 2 m) F[-3 + m, -3 + k, -2 + j, -1 + p] +
  (-7 + 2 m) (-5 + 2 m) (-9 + 4 k + 2 m) F[-2 + m, -2 + k, -2 + j, -1 + p] +
  (-7 + 2 m) (-5 + 2 m) (-3 + 2 m) F[-1 + m, -1 + k, -2 + j, -1 + p];

```

In[19]:= **recf[[1, 2, 1, 2]] /. m → m - 1 // Simplify**

Out[19]=  $(-7 + 2m)(-4(-2 + k)(-4 + k + m)F[-3 + m, -3 + k, -2 + j, p] +$   
 $4(k - m)(-2 + m)F[-3 + m, -2 + k, -2 + j, -1 + p] -$   
 $4(k - m)(-2 + m)F[-3 + m, -2 + k, -2 + j, p] - (-5 + 2m)(-9 + 4k + 2m)$   
 $F[-2 + m, -2 + k, -2 + j, p] - (-3 + 2k)(-5 + 2m)F[-2 + m, -2 + k, -1 + j, p] +$   
 $2(k - m)(-5 + 2m)F[-2 + m, -1 + k, -2 + j, -1 + p] +$   
 $2(-k + m)(-5 + 2m)F[-2 + m, -1 + k, -2 + j, p] +$   
 $2(k - m)(-5 + 2m)F[-2 + m, -1 + k, -1 + j, -1 + p] +$   
 $2(-k + m)(-5 + 2m)F[-2 + m, -1 + k, -1 + j, p] -$   
 $(-5 + 2m)(-3 + 2m)F[-1 + m, -1 + k, -2 + j, p] -$   
 $(-5 + 2m)(-3 + 2m)F[-1 + m, -1 + k, -1 + j, p])$

In[20]:= **fj[m\_, k\_, j\_, p\_] :=**

$(-7 + 2m)(-4(-2 + k)(-4 + k + m)F[-3 + m, -3 + k, -2 + j, p] + 4(k - m)(-2 + m)$   
 $F[-3 + m, -2 + k, -2 + j, -1 + p] - 4(k - m)(-2 + m)F[-3 + m, -2 + k, -2 + j, p] -$   
 $(-5 + 2m)(-9 + 4k + 2m)F[-2 + m, -2 + k, -2 + j, p] -$   
 $(-3 + 2k)(-5 + 2m)F[-2 + m, -2 + k, -1 + j, p] +$   
 $2(k - m)(-5 + 2m)F[-2 + m, -1 + k, -2 + j, -1 + p] + 2(-k + m)(-5 + 2m)$   
 $F[-2 + m, -1 + k, -2 + j, p] + 2(k - m)(-5 + 2m)F[-2 + m, -1 + k, -1 + j, -1 + p] +$   
 $2(-k + m)(-5 + 2m)F[-2 + m, -1 + k, -1 + j, p] - (-5 + 2m)(-3 + 2m)$   
 $F[-1 + m, -1 + k, -2 + j, p] - (-5 + 2m)(-3 + 2m)F[-1 + m, -1 + k, -1 + j, p]);$

In[21]:= **fj[m, m, j, p]**

Out[21]=  $(-7 + 2m)(-4(-2 + m)(-4 + 2m)F[-3 + m, -3 + m, -2 + j, p] -$   
 $(-5 + 2m)(-9 + 6m)F[-2 + m, -2 + m, -2 + j, p] -$   
 $(-5 + 2m)(-3 + 2m)F[-2 + m, -2 + m, -1 + j, p] - (-5 + 2m)(-3 + 2m)$   
 $F[-1 + m, -1 + m, -2 + j, p] - (-5 + 2m)(-3 + 2m)F[-1 + m, -1 + m, -1 + j, p])$

In[22]:= **fj[m, m - 1, j, p]**

Out[22]=  $(-7 + 2m)(-4(-3 + m)(-5 + 2m)F[-3 + m, -4 + m, -2 + j, p] -$   
 $4(-2 + m)F[-3 + m, -3 + m, -2 + j, -1 + p] + 4(-2 + m)F[-3 + m, -3 + m, -2 + j, p] -$   
 $(-5 + 2m)(-9 + 4(-1 + m) + 2m)F[-2 + m, -3 + m, -2 + j, p] -$   
 $(-3 + 2(-1 + m))(-5 + 2m)F[-2 + m, -3 + m, -1 + j, p] -$   
 $2(-5 + 2m)F[-2 + m, -2 + m, -2 + j, -1 + p] + 2(-5 + 2m)F[-2 + m, -2 + m, -2 + j, p] -$   
 $2(-5 + 2m)F[-2 + m, -2 + m, -1 + j, -1 + p] + 2(-5 + 2m)F[-2 + m, -2 + m, -1 + j, p] -$   
 $(-5 + 2m)(-3 + 2m)F[-1 + m, -2 + m, -2 + j, p] -$   
 $(-5 + 2m)(-3 + 2m)F[-1 + m, -2 + m, -1 + j, p])$

In[23]:= **dfj[m\_, k\_, j\_, p\_] := fj[m, k, j + 1, p] - fj[m, k, j, p];**

In[24]:= **recf[[1, 2, 2, 2]] /. m → m - 1 // Simplify**

Out[24]=  $-4(-3 + k)(-2 + k)(-5 + 2m)F[-4 + m, -4 + k, -2 + j, -1 + p] -$   
 $4(-2 + k)(-7 + 2m)(-6 + k + 2m)F[-3 + m, -3 + k, -2 + j, -1 + p] +$   
 $4(-2 + m)(-k + m)(-7 + 2m)F[-3 + m, -2 + k, -2 + j, -1 + p] -$   
 $(-7 + 2m)(-5 + 2m)(-9 + 4k + 2m)F[-2 + m, -2 + k, -2 + j, -1 + p] +$   
 $2(-k + m)(-7 + 2m)(-5 + 2m)F[-2 + m, -1 + k, -2 + j, -1 + p] -$   
 $(-7 + 2m)(-5 + 2m)(-3 + 2m)F[-1 + m, -1 + k, -2 + j, -1 + p]$

```
In[25]:= fp[m_, k_, j_, p_] := -4 (-3 + k) (-2 + k) (-5 + 2 m) F[-4 + m, -4 + k, -2 + j, -1 + p] -
      4 (-2 + k) (-7 + 2 m) (-6 + k + 2 m) F[-3 + m, -3 + k, -2 + j, -1 + p] +
      4 (-2 + m) (-k + m) (-7 + 2 m) F[-3 + m, -2 + k, -2 + j, -1 + p] -
      (-7 + 2 m) (-5 + 2 m) (-9 + 4 k + 2 m) F[-2 + m, -2 + k, -2 + j, -1 + p] +
      2 (-k + m) (-7 + 2 m) (-5 + 2 m) F[-2 + m, -1 + k, -2 + j, -1 + p] -
      (-7 + 2 m) (-5 + 2 m) (-3 + 2 m) F[-1 + m, -1 + k, -2 + j, -1 + p];
```

```
In[26]:= fp[m, m, j, p]
```

```
Out[26]:= -4 (-3 + m) (-2 + m) (-5 + 2 m) F[-4 + m, -4 + m, -2 + j, -1 + p] -
      4 (-2 + m) (-7 + 2 m) (-6 + 3 m) F[-3 + m, -3 + m, -2 + j, -1 + p] -
      (-7 + 2 m) (-5 + 2 m) (-9 + 6 m) F[-2 + m, -2 + m, -2 + j, -1 + p] -
      (-7 + 2 m) (-5 + 2 m) (-3 + 2 m) F[-1 + m, -1 + m, -2 + j, -1 + p]
```

```
In[27]:= fp[m, m - 1, j, p] // Simplify
```

```
Out[27]:= -4 (-4 + m) (-3 + m) (-5 + 2 m) F[-4 + m, -5 + m, -2 + j, -1 + p] -
      4 (-3 + m) (-7 + 2 m) (-7 + 3 m) F[-3 + m, -4 + m, -2 + j, -1 + p] +
      4 (-2 + m) (-7 + 2 m) F[-3 + m, -3 + m, -2 + j, -1 + p] -
      (-7 + 2 m) (-5 + 2 m) (-13 + 6 m) F[-2 + m, -3 + m, -2 + j, -1 + p] +
      2 (-7 + 2 m) (-5 + 2 m) F[-2 + m, -2 + m, -2 + j, -1 + p] -
      (-7 + 2 m) (-5 + 2 m) (-3 + 2 m) F[-1 + m, -2 + m, -2 + j, -1 + p]
```

```
In[28]:= dfp[m_, k_, j_, p_] := fp[m, k, j, p + 1] - fp[m, k, j, p];
```

## The key identity

```
In[29]:= lhsf
```

```
Out[29]:= 4 (-3 + k) (-2 + k) (-5 + 2 m) F[-4 + m, -4 + k, -2 + j, -1 + p] +
      4 (-2 + k) (-7 + 2 m) (-6 + k + 2 m) F[-3 + m, -3 + k, -2 + j, -1 + p] +
      (-7 + 2 m) (-5 + 2 m) (-9 + 4 k + 2 m) F[-2 + m, -2 + k, -2 + j, -1 + p] +
      (-7 + 2 m) (-5 + 2 m) (-3 + 2 m) F[-1 + m, -1 + k, -2 + j, -1 + p]
```

```
In[30]:= 4 (-3 + k) (-2 + k) (-5 + 2 m) F[-4 + m, -4 + k, -2 + j, -1 + p] +
      4 (-2 + k) (-7 + 2 m) (-6 + k + 2 m) F[-3 + m, -3 + k, -2 + j, -1 + p] +
      (-7 + 2 m) (-5 + 2 m) (-9 + 4 k + 2 m) F[-2 + m, -2 + k, -2 + j, -1 + p] +
      (-7 + 2 m) (-5 + 2 m) (-3 + 2 m) F[-1 + m, -1 + k, -2 + j, -1 + p] ==
      dfj[m, k, j, p] + dfp[m, k, j, p] /. F -> f // FullSimplify
```

```
Out[30]= True
```

FullSimplify checks the identity as an identity of meromorphic functions in the variables  $m, k, j, p$ . So we now know the identity at points of continuity of the meromorphic functions.

```
In[31]:= Table[4 (-3 + k) (-2 + k) (-5 + 2 m) F[-4 + m, -4 + k, -2 + j, -1 + p] +
      4 (-2 + k) (-7 + 2 m) (-6 + k + 2 m) F[-3 + m, -3 + k, -2 + j, -1 + p] +
      (-7 + 2 m) (-5 + 2 m) (-9 + 4 k + 2 m) F[-2 + m, -2 + k, -2 + j, -1 + p] +
      (-7 + 2 m) (-5 + 2 m) (-3 + 2 m) F[-1 + m, -1 + k, -2 + j, -1 + p] ==
      dfj[m, k, j, p] + dfp[m, k, j, p] /. F -> f // FullSimplify, {j, -2, 2}, {p, -2, 2}]

Out[31]= {{True, True, True, True, True},
  {True, True, True, True, True}, {True, True, True, True, True},
  {True, True, True, True, True}, {True, True, True, True, True}}
```

Let  $m \geq k \geq 2$ . The key identity holds. We sum the key identity over all  $j$  and  $p$ . There are only finitely many terms. The right hand side cancels by telescoping. We get a recursion for  $\text{sum}[m, k]$ , where  $\text{sum}[m, k]$  is the sum over  $j, p$  of  $f[m, k, j, p]$ . We check below that our guessed answer  $fF$  satisfies the same recursion. So we get a proof of our guess as soon as we have enough initial cases checked. Our guess:

```
In[32]:= fF[m_, k_, ___] := (-1)^m (2 m + 1) / (2 (m - k) + 1)
```

```
In[33]:= lhsf /. F -> fF
```

```
Out[33]= 
$$\frac{4 (-1)^{-4+m} (-3 + k) (-2 + k) (1 + 2 (-4 + m)) (-5 + 2 m)}{1 + 2 (-k + m)} +$$


$$\frac{(-1)^{-1+m} (1 + 2 (-1 + m)) (-7 + 2 m) (-5 + 2 m) (-3 + 2 m)}{1 + 2 (-k + m)} +$$


$$\frac{4 (-1)^{-3+m} (-2 + k) (1 + 2 (-3 + m)) (-7 + 2 m) (-6 + k + 2 m)}{1 + 2 (-k + m)} +$$


$$\frac{(-1)^{-2+m} (1 + 2 (-2 + m)) (-7 + 2 m) (-5 + 2 m) (-9 + 4 k + 2 m)}{1 + 2 (-k + m)}$$

```



In[34]:= **Simplify[%]**

Out[34]= 0

## Put

In[35]:= **rel[k\_] = lhsf /. F[a\_, b\_, \_\_] → sum[a, b]**

Out[35]=  $4(-3+k)(-2+k)(-5+2m) \text{sum}[-4+m, -4+k] +$   
 $4(-2+k)(-7+2m)(-6+k+2m) \text{sum}[-3+m, -3+k] +$   
 $(-7+2m)(-5+2m)(-9+4k+2m) \text{sum}[-2+m, -2+k] +$   
 $(-7+2m)(-5+2m)(-3+2m) \text{sum}[-1+m, -1+k]$

## The rel[k] vanish for $m \geq k \geq 2$ .

In[36]:= **rel[5]**

Out[36]=  $24(-5+2m) \text{sum}[-4+m, 1] + 12(-7+2m)(-1+2m) \text{sum}[-3+m, 2] +$   
 $(-7+2m)(-5+2m)(11+2m) \text{sum}[-2+m, 3] +$   
 $(-7+2m)(-5+2m)(-3+2m) \text{sum}[-1+m, 4]$

In[37]:= **rel[4]**

Out[37]=  $8(-5+2m) \text{sum}[-4+m, 0] + 8(-7+2m)(-2+2m) \text{sum}[-3+m, 1] +$   
 $(-7+2m)(-5+2m)(7+2m) \text{sum}[-2+m, 2] + (-7+2m)(-5+2m)(-3+2m) \text{sum}[-1+m, 3]$

In[38]:= **rel[3]**

Out[38]=  $4(-7+2m)(-3+2m) \text{sum}[-3+m, 0] + (-7+2m)(-5+2m)(3+2m) \text{sum}[-2+m, 1] +$   
 $(-7+2m)(-5+2m)(-3+2m) \text{sum}[-1+m, 2]$

In[39]:= **rel[2]**

Out[39]=  $(-7+2m)(-5+2m)(-1+2m) \text{sum}[-2+m, 0] + (-7+2m)(-5+2m)(-3+2m) \text{sum}[-1+m, 1]$

Recall that fF satisfies the same recurrence. Indeed:

```
In[40]:= Table[rel[i] /. sum -> fF, {i, 2, 4}]
```

$$\text{Out[40]} = \left\{ \frac{(-1)^{-1+m} (1+2(-1+m)) (-7+2m) (-5+2m) (-3+2m)}{1+2(-2+m)} + \right. \\ (-1)^{-2+m} (-7+2m) (-5+2m) (-1+2m), \\ 4(-1)^{-3+m} (-7+2m) (-3+2m) + \frac{(-1)^{-1+m} (1+2(-1+m)) (-7+2m) (-5+2m) (-3+2m)}{1+2(-3+m)} + \\ \frac{(-1)^{-2+m} (1+2(-2+m)) (-7+2m) (-5+2m) (3+2m)}{1+2(-3+m)}, \\ 8(-1)^{-4+m} (-5+2m) + \frac{(-1)^{-1+m} (1+2(-1+m)) (-7+2m) (-5+2m) (-3+2m)}{1+2(-4+m)} + \\ \frac{8(-1)^{-3+m} (1+2(-3+m)) (-7+2m) (-2+2m)}{1+2(-4+m)} + \\ \left. \frac{(-1)^{-2+m} (1+2(-2+m)) (-7+2m) (-5+2m) (7+2m)}{1+2(-4+m)} \right\}$$

```
In[41]:= % // Simplify
```

```
Out[41]= {0, 0, 0}
```

If we know  $\text{sum}[m-2,0]$  for  $m \geq 2$  then  $\text{rel}[2]=0$  gives  $\text{sum}[m-1,1]$  for  $m \geq 2$ . And so on.

So we actually only need the case  $k=0$  to conclude that  $\text{sum}[m,k]$  equals  $\text{fF}[m,k]$  for  $m \geq k \geq 0$ . Mathematica confirms the case  $k=0$  :

```
In[42]:= f[m, 0, 0, p]
```

$$\text{Out[42]} = \frac{(-1)^p \text{Binomial}[m, p]^2 \text{Gamma}\left[\frac{1}{2} + m - p\right] \text{Gamma}[1 + p]}{\text{Gamma}\left[\frac{1}{2} + m\right]}$$

```
In[43]:= Sum[f[m, 0, 0, p], {p, 0, m}]
```

```
Out[43]= (-1)^m
```

```
In[44]:= fF[m, 0]
```

```
Out[44]= (-1)^m
```

## A proof for the case k=0:

In[45]:= **f[m, 0, 0, p]**

$$\text{Out[45]} = \frac{(-1)^p \text{Binomial}[m, p]^2 \text{Gamma}\left[\frac{1}{2} + m - p\right] \text{Gamma}[1 + p]}{\text{Gamma}\left[\frac{1}{2} + m\right]}$$

In[46]:= **rec0 = FindRecurrence[f[m, 0, 0, p], m, p]**

$$\text{Out[46]} = \left\{ (-1 + 2m)(1 + 2m) F[m, -2 + p] + (-1 + 2m)(1 + 2m) F[1 + m, -2 + p] = \right. \\ \Delta_p \left[ 4m^2 F[-1 + m, -2 + p] - (-1 + 2m)(1 + 2m) F[m, -2 + p] + \right. \\ (-1 + 2m)(1 + 2m) F[m, -1 + p] - (-1 + 2m)(1 + 2m) F[1 + m, -2 + p] - \\ \left. (-1 + 2m)(1 + 2m) F[1 + m, -1 + p] \right] \left. \right\}$$

In[47]:= **(-1 + 2m)(1 + 2m) fF[m, 0, 0, -2 + p] +**  
**(-1 + 2m)(1 + 2m) fF[1 + m, 0, 0, -2 + p] // Simplify**

Out[47]= **0**

In[48]:= **Sum[f[1, 0, 0, p], {p, 0, 1}]**

Out[48]= **-1**

In[49]:= **fF[1, 0]**

Out[49]= **-1**

In[50]:= **rec0[[1, 1]] /. F[a\_, b\_] -> ff[a, 0, 0, b]**

$$\text{Out[50]} = (-1 + 2m)(1 + 2m) ff[m, 0, 0, -2 + p] + (-1 + 2m)(1 + 2m) ff[1 + m, 0, 0, -2 + p]$$

In[51]:= **lhs0[m\_, p\_] =**

$$(-1 + 2m)(1 + 2m) ff[m, 0, 0, -2 + p] + (-1 + 2m)(1 + 2m) ff[1 + m, 0, 0, -2 + p]$$

$$\text{Out[51]} = (-1 + 2m)(1 + 2m) ff[m, 0, 0, -2 + p] + (-1 + 2m)(1 + 2m) ff[1 + m, 0, 0, -2 + p]$$

In[52]:= **rec0[[1, 2, 2]] /. F[a\_, b\_] -> ff[a, 0, 0, b]**

$$\text{Out[52]} = 4m^2 ff[-1 + m, 0, 0, -2 + p] - (-1 + 2m)(1 + 2m) ff[m, 0, 0, -2 + p] + \\ (-1 + 2m)(1 + 2m) ff[m, 0, 0, -1 + p] - (-1 + 2m)(1 + 2m) ff[1 + m, 0, 0, -2 + p] - \\ (-1 + 2m)(1 + 2m) ff[1 + m, 0, 0, -1 + p]$$

In[53]:= **fp0[m\_, p\_] = 4m^2 ff[-1 + m, 0, 0, -2 + p] -**

$$(-1 + 2m)(1 + 2m) ff[m, 0, 0, -2 + p] + (-1 + 2m)(1 + 2m) ff[m, 0, 0, -1 + p] -$$

$$(-1 + 2m)(1 + 2m) ff[1 + m, 0, 0, -2 + p] - (-1 + 2m)(1 + 2m) ff[1 + m, 0, 0, -1 + p]$$

$$\text{Out[53]} = 4m^2 ff[-1 + m, 0, 0, -2 + p] - (-1 + 2m)(1 + 2m) ff[m, 0, 0, -2 + p] + \\ (-1 + 2m)(1 + 2m) ff[m, 0, 0, -1 + p] - (-1 + 2m)(1 + 2m) ff[1 + m, 0, 0, -2 + p] - \\ (-1 + 2m)(1 + 2m) ff[1 + m, 0, 0, -1 + p]$$

In[54]:= **Table[fp0[m, p] /. ff -> f, {p, 0, 1}]**

Out[54]= **{0, 0}**

In[55]:= **lhs0[m, p] == fp0[m, p + 1] - fp0[m, p] /. ff -> f // FullSimplify**

Out[55]= **True**

```
In[56]:= Table[lhs0[m, p] == fp0[m, p + 1] - fp0[m, p] /. ff → f // FullSimplify, {p, 0, 2}]  
Out[56]= {True, True, True}
```

---

Done.
